# Supplementary material for: Beyond the heat: The mental health toll of temperature and humidity in India
Source: arXiv:2503.08761 source file (2025-03-11)
Supplement: Supplementary file 1 [file AppendixA.tex]

\subsection*{Appendix B: Summary statistics - Dry bulb temperature}
% !TEX spellcheck = en_US
\setcounter{table}{0} 

\begin{table}[h!]
	\caption{\label{sumstats07}Summary statistics - Dry bulb temperature}
	\small
	\centering
	\begin{tabular}{lrrrr}
		\midrule
		\midrule 
                                 & Mean & SD   & Min & Max \\
                                 \midrule
    Dry bulb temperature &       29.87&        4.52&          11&          43\\
    & & & & \\
\# Days \textless 23.5°C&        3.87&        8.18&           0&          30\\
\# Days 23.5°C-25°C&        1.73&        3.43&           0&          24\\
\# Days 25°C-26.5°C&        2.20&        3.71&           0&          30\\
\# Days 26.5°C-28°C&        2.87&        3.87&           0&          28\\
\# Days 28°C-29.5°C&        3.74&        5.05&           0&          23\\
\# Days 29.5°C-31°C&        3.43&        4.43&           0&          25\\
\# Days 31°C-32.5°C&        3.11&        4.31&           0&          21\\
\# Days 32.5°C-34°C&        2.71&        3.77&           0&          19\\
\# Days 34°C-35.5°C&        2.62&        4.11&           0&          19\\
\# Days 35.5°C-37°C&        2.09&        3.79&           0&          19\\
\# Days $\geq$ 37°C&        1.62&        4.12&           0&          28\\
    & & & & \\
Heat wave ( days $\geq$ 37°)&        0.16&        0.36&           0&           1\\
Heat wave ($\geq$ 3 days $\geq$ 37°)&        0.14&        0.34&           0&           1\\
\# Consecutive days $\geq$ 37°&        1.11&        3.10&           0&          26\\
    & & & & \\
\# Days \textless 25.5°C&        6.28&       10.25&           0&          30\\
\# Days 25.5.5°C-27°C&        2.39&        3.77&           0&          30\\
\# Days 27°C-28.5°C&        3.15&        4.17&           0&          28\\
\# Days 28.5°C-30°C&        3.86&        5.18&           0&          26\\
\# Days 30°C-31.5°C&        3.19&        4.03&           0&          25\\
\# Days 31.5°C-33°C&        3.06&        4.09&           0&          20\\
\# Days 33°C-34.5°C&        2.67&        3.96&           0&          20\\
\# Days 34.5°C-36°C&        2.48&        4.01&           0&          19\\
\# Days 36°C-37.5°C&        1.82&        3.61&           0&          20\\
\# Days 37.5°C-39°C&        0.78&        2.07&           0&          15\\
\# Days $\geq$ 39°C&        0.32&        1.55&           0&          20\\
    & & & & \\
Heat wave ($\geq$ 2 days $\geq$ 39°)&        0.05&        0.21&           0&           1\\
Heat wave ($\geq$ 3 days $\geq$ 39°)&        0.04&        0.19&           0&           1\\
\# Consecutive days $\geq$ 39°&        0.23&        1.04&           0&          13\\
\hline
Observations        &       30300&            &            &            \\
\hline\hline
	\multicolumn{5}{p{8cm}}{}   

	\end{tabular}
\end{table}
